# Supplementary material for: Shape of the Cloak: Formal Analysis of Clock Skew-Based Intrusion Detection System in Controller Area Networks
Source: arXiv:1807.09432 source file (2019-01-24)
Supplement: Supplementary file 1 [file appendix_attack_on_correlation_detector.tex]

\subsection{Cloaking Attack on Correlation Detector}
\label{sec:cloaking_on_correlation_analysis}
%\textcolor{red}{We observed that an ECU transmits multiple messages, however, it is not always true that these messages are consecutively transmitted and received. (See Section \ref{sec:evaluation_attack_on_correlation}.) Hence, the sibling message may not exist for some messages, and the correlation detector is not applicable such a case.}
In practice, it is not uncommon for an ECU to transmit multiple messages with the same or different periods and priorities (i.e., sibling messages). %, and it is not uncommon for an ECU to transmit multiple messages consecutively
If the spoofed message has a sibling message with the same period and highly correlated offsets, the correlation detector can be deployed as the secondary countermeasure. 
Before introducing the cloaking attack on the correlation detector, let us discuss why two messages consecutively transmitted and consecutively received are more likely to have high correlation in average offsets.
Due to space constraints, we focus on the NTP-based IDS, but the same logic is applicable to the state-of-the-art IDS.

%Since the two messages are consecutively transmitted and received, it is reasonable to assume that each pair 

Denote the $i$-th message in the $k$-th batch for messages $v$ and $w$ as $v_{k,i}$ and $w_{k,i}$, which are transmitted at $t_{k,i}^{(v)}$ and $t_{k,i}^{(w)}$, respectively.\footnote{This is another requirement for two messages to be highly correlated: the two consecutively transmitted messages needs to be processed as simultaneously as the $i$-th message in the $k$-th batch.}
Without loss of generality, suppose that $w_{k,i}$ is transmitted right after $v_{k,i}$.
Let $\Delta t$ be the transmission duration of each message $v$, which is constant, given the fixed message length and CAN bus speed. 
Hence, we have $t_{k,i}^{(w)}=t_{k,i}^{(v)}+\Delta t$.

Let us consider the first case where $v_{k,i}$ and $w_{k,i}$ are received consecutively at $a_{k,i}^{(v)}$ and $a_{k,i}^{(w)}$, which means no other messages with higher priority IDs are received between $a_{k,i}^{(v)}$ and $a_{k,i}^{(w)}$ due to arbitration. 
For simplicity, we assume constant network delays for both messages (denoted as $d_v$ and $d_w$, respectively), and ignore quantization noise at the receiver. 
Therefore we have $a_{k,i}^{(w)}=a_{k,i}^{(v)}+\Delta t + (d_w - d_v)$.

In the NTP-based IDS, the estimated average offset for messages $v$ and $w$ in the $k$-th batch are  
\begin{eqnarray}
\nonumber
O_{avg}^{(v)}[k] &=& T-\frac{1}{N}\left( a_{k,N}^{(v)} - a_{k,0}^{(v)} \right) \\
\nonumber
&=& -O^{(v)} - \frac{1}{N}\left(\epsilon_{k,N}^{(v)}-\epsilon_{k,0}^{(v)}\right) \\
O_{avg}^{(w)}[k] &=& T-\frac{1}{N}\left( a_{k,N}^{(w)} - a_{k,0}^{(w)} \right) = O_{avg}^{(v)}[k]. \label{eq:cloaking_correlation_same_avg_offset}
\end{eqnarray}
Since $O_{avg}^{(v)}[k]$ and $O_{avg}^{(w)}[k]$ are the $k$-th realizations of the random variables $O_{avg}^{(v)}$ and $O_{avg}^{(w)}$, respectively, Eq.~(\ref{eq:cloaking_correlation_same_avg_offset}) implies $O_{avg}^{(w)}=O_{avg}^{(v)}$, and thus their correlation coefficient $\rho$ is as high as $1$.
In general, as along as the two messages are received with a constant delay (consecutive reception is a special case), they will have high correlation. 
In practice, however, the correlation would slightly decrease due to network delay variations and quantization noise at the receiver.

Next we examine the second case in which messages with higher priority IDs are received in between the two messages.
Let the arbitration delay be $d_{k,i}\geq 0$, and thus $a_{k,i}^{(w)}=a_{k,i}^{(v)}+\Delta t + (d_w - d_v) + d_{k,i}$.
Then we have
\begin{equation}
O_{avg}^{(w)}[k] = O_{avg}^{(v)}[k] - \frac{1}{N}(d_{k,N}-d_{k,0}),
\end{equation}
where the second term may be considered as the $k$-th realization of a random variable $D$, independent of $O_{avg}^{(v)}$ and $O_{avg}^{(w)}$. 
Therefore, we have $O_{avg}^{(w)}=O_{avg}^{(v)} + D$, and 
\begin{equation*}
\rho \left(O_{avg}^{(v)}, O_{avg}^{(w)} \right) = \frac{\sqrt{Var (O_{avg}^{(v)})}}{\sqrt{Var(O_{avg}^{(v)}) + Var(D)}} < 1.
\end{equation*}
As a result, depending on the variance of arbitration delay, the correlation in the second case may be much smaller than $1$.

On the other hand, if two messages are transmitted from different ECUs, we have $O_{avg}^{(w)}[k]=-O^{(w)}- \frac{1}{N}\left(\epsilon_{k,N}^{(w)}-\epsilon_{k,0}^{(w)}\right)$. 
Since $\{\epsilon_{k,i}^{(v)}\}$ and $\{\epsilon_{k,i}^{(w)}\}$ are independent, $O_{avg}^{(w)}$ is also independent of $O_{avg}^{(v)}$, which implies $\rho\approx 0$.
The above analysis is supported by our hardware evaluation (Section \ref{sec:evaluation_attack_on_correlation}).

Hence, the attacker adopts the following strategy to thwart the correlation detector. Before the attack, the attacker observes the targeted message for a certain duration and identifies any sibling messages. 
During the attack, the strong attacker-controlled ECU A transmits %begins transmitting 
a spoofed message immediately 
after a sibling message is received. %completed. 
Since the spoofed and sibling messages are transmitted almost consecutively, their average offsets
%Since the transmission from ECU A begins once the sibling message transmission ends, the average offset of the targeted and sibling messages
will be equivalent and highly correlated (Eq. (\ref{eq:cloaking_correlation_same_avg_offset})).
Note that Eq. (\ref{eq:cloaking_correlation_same_avg_offset}) also implies that their estimated accumulated offsets and clock skews will be equivalent, thus bypassing the clock skew detector at the same time.

%To bypass the correlation detector, the attack strategy is also rather simple: \textit{the impersonating ECU transmits the spoofed message immediately after it observes a sibling message of the spoofed message.}
%\cmt{Explain that this is to make sure that the two messages are consecutively received by the IDS with a constant delay.}
%According to our previous discussion, this strategy should lead to high correlation between the two messages.
%In fact, \rev{it also ensures that they have very close clock skews (Eq.~(\ref{eq:cloaking_correlation_same_avg_offset})), and can bypass the clock skew detector.}
